# Supplementary material for: GADMM: Fast and Communication Efficient Framework for Distributed Machine Learning
Source: arXiv:1909.00047 source file (2020-03-24)
Supplement: Supplementary file 1 [file appendix_C.tex]

\section{Proof of Theorem~\ref{convRateProof}: Convergence Rate of GADMM}
\label{ConvRate11}

%The convergence rate of Gauss-Seidel ADMM for sum of two separable convex functions has been studied in~\citep{lions1979splitting,he20121,he2015non}. In particular, \citep{he20121} shows a convergence rate of $O(1/k)$. Moreover, \citep{deng2017parallel} improves that results and shows a convergence rate of $o(1/k)$. In this section, we leverage and extend the proof of $o(1/k)$ convergence rate in \cite[Sec. 5]{deng2017parallel} to showing that GADMM achieves the same convergence~rate.
\if0

\colr{Consider the notation in \eqref{notation} and the definition of $\bbr_{n,n+1}^{k+1}$, we can write the result  in 
\eqref{mainIneq2} as follows
\begin{align}\label{rate:first}
\|\bbw_{k+1}-\bbw^\star\|^2_\bbH\leq &\|\bbw_{k}-\bbw^\star\|^2_\bbH-
\frac{1}{\rho}\sum_{n=1}^{N-1} \norm{\lamb_{n}^{k+1} - \lamb_{n}^{k}}^2\nonumber 
\\
&-\sum_{n\in {\cal N}_h\setminus\{1\}} \rho\norm{ \boldsymbol{\theta}_{n-1}^{k+1} -  \boldsymbol{\theta}_{n-1}^k}^2-\sum_{n\in {\cal N}_h}\rho\norm{ \boldsymbol{\theta}_{n+1}^{k+1} -  \boldsymbol{\theta}_{n+1}^k}^2.
\end{align}
Further, from the definition of $\bbw_k$ and the notation in \eqref{notation}, we can write
\begin{align}\label{rate:2}
\|\bbw_{k+1}-\bbw^\star\|^2_\bbH\leq &\|\bbw_{k}-\bbw^\star\|^2_\bbH-\|\bbw_{k+1}-\bbw_{k}\|^2_\bbH.
\end{align}
The result in \eqref{rate:2} shows that the iterate sequence $\bbw_k$ obtained by the GADMM algorithm is strictly contractive. This implies that the sequence $\|\bbw_{k}-\bbw^\star\|^2_\bbH$ is monotonically decreasing as $k\rightarrow\infty$. This result implies the convergence of the iterates $\bbw_k$ from the contraction methods \citep{He1997}. 
To prove the convergence rate using the Lemma \ref{lemma:convRate}, we define the sequence $a_k:=\|\bbw_{k+1}-\bbw^\star\|^2_\bbH$. In order to apply the results of Lemma \ref{lemma:convRate}, we need to prove that 
i) $a_k$ sequence is positive which is trivial from the definition,
ii) $a_k$ is monotonically non-increasing,
iii) and $a_k$ is summable.}
For the sequence ${\textbf w}_n$, I think its difficult to prove the third point, hence we cannot use Lemma 3. We can prove these three properties for ${\textbf w}_n^k$
Let us define ${\textbf w}_n$ for all $n \in {\cal N}_t$ and $\bbH$ as follows:
\begin{align}\label{definitions}
{\textbf w}_n:=\begin{bmatrix} 
\boldsymbol{\theta}_n\\
-\lamb_{n-1}\\
\lamb_{n}\\
\end{bmatrix}
,\bbH:=\begin{bmatrix} 
\rho \bbA_n^T\bbA_n& \\
& \frac{1}{\rho}\bbI\\
&& \frac{1}{\rho}\bbI\\
\end{bmatrix},
\end{align}

\fi

Let us define ${\textbf w}_n$ for all $n \in {\cal N}_t$ and $\bbH$ as follows:
\begin{align}\label{definitions}
{\textbf w}_n:=\begin{bmatrix} 
\boldsymbol{\theta}_n\\
-\lamb_{n-1}\\
\lamb_{n}\\
\end{bmatrix}
,\bbH:=\begin{bmatrix} 
\rho \bbA_n^T\bbA_n& \\
& \frac{1}{\rho}\bbI\\
&& \frac{1}{\rho}\bbI\\
\end{bmatrix},
\end{align}

where, $\bbA_{n \in  {\cal N}_t} \in \mathbb{R}^{(N-1)\times d}$ is the sub-matrix of the $n$-th element when the constraints in \eqref{com_admm_c1} are written in the matrix form, and $\bbI \in \mathbb{R}^{(N-1)\times(N-1)}$ is the identity matrix.
From the definitions in \eqref{definitions}, it holds that
\begin{align}
\!\!\!\!\!\!\!\!\sum_{n \in {\cal N}_t}\Big[\!\norm{{\textbf w}_n^{k} \!-\!  {\textbf w}_n^\star}_\bbH^2\!-\norm{ {\textbf w}_n^{k+1} \!\!-\!  {\textbf w}_n^\star}_\bbH^2\Big]&\!\!=\!\!\sum_{n} 1/\rho\left(\norm{ \lamb_n^{k}-\lamb_n^\star}^2-\norm{\lamb_n^{k+1}-\lamb_n^\star}^2\right)\nonumber
\\
&\quad+\!\!\sum_{n\in {\cal N}_t}\rho\left(\norm{\boldsymbol{\theta}_{n}^{k} -  \boldsymbol{\theta}^\star}^2- \norm{\boldsymbol{\theta}_{n}^{k+1} -  \boldsymbol{\theta}^\star}^2\right)
\label{convRateEq1}
\end{align}
where $\norm{\bbx}_{\bbH}^2=\ip{\bbx,\bbH\bbx}$. However, the following holds true for the second term on the right hand side of \eqref{convRateEq1}
\begin{align}\label{convRateEq2}
\sum_{n\in {\cal N}_t}\rho\left(\norm{\boldsymbol{\theta}_{n}^{k} -  \boldsymbol{\theta}^\star}^2- \norm{\boldsymbol{\theta}_{n}^{k+1} -  \boldsymbol{\theta}^\star}^2\right)
\!\!=\!\!\!&\!\!\!\!\sum_{n\in {\cal N}_h\setminus\{1\}}\rho\left( \norm{\boldsymbol{\theta}_{n-1}^{k} -  \boldsymbol{\theta}^\star}^2- \norm{\boldsymbol{\theta}_{n-1}^{k+1} -  \boldsymbol{\theta}^\star}^2\right)\nonumber
\\
&\quad\quad+\sum_{n\in {\cal N}_h}\rho\left(\norm{\boldsymbol{\theta}_{n+1}^{k} -  \boldsymbol{\theta}^\star}^2-\norm{ \boldsymbol{\theta}_{n+1}^{k+1} -  \boldsymbol{\theta}^\star}^2\right).
\end{align}
Therefore, the right hand side of \eqref{convRateEq1} reduces to 
\begin{align}\label{convRateEq3}
\!\!\!\!\!\!\!\!\sum_{n \in {\cal N}_t}\Big[\!\norm{{\textbf w}_n^{k} \!-\!  {\textbf w}_n^\star}_\bbH^2\!-\norm{ {\textbf w}_n^{k+1} \!\!-\!  {\textbf w}_n^\star}_\bbH^2\Big]&\!\!=\!\!\sum_{n} 1/\rho\left(\norm{ \lamb_n^{k}-\lamb_n^\star}^2-\norm{\lamb_n^{k+1}-\lamb_n^\star}^2\right)
\\
&\quad+\sum_{n\in {\cal N}_h\setminus\{1\}}\rho\left( \norm{\boldsymbol{\theta}_{n-1}^{k} -  \boldsymbol{\theta}^\star}^2- \norm{\boldsymbol{\theta}_{n-1}^{k+1} -  \boldsymbol{\theta}^\star}^2\right)\nonumber
\\
&\quad\quad+\sum_{n\in {\cal N}_h}\rho\left(\norm{\boldsymbol{\theta}_{n+1}^{k} -  \boldsymbol{\theta}^\star}^2-\norm{ \boldsymbol{\theta}_{n+1}^{k+1} -  \boldsymbol{\theta}^\star}^2\right). \nonumber
\end{align}
However, from \eqref{mainIneq} in the proof of Theorem \ref{theorem}, it holds that all the three terms on the right hand side of equality in \eqref{convRateEq3} are monotonically non-increasing. Hence,  the term $\sum_{n \in {\cal N}_t}\norm{{\textbf w}_n^{k+1} -  {\textbf w}_n^{k}}_\bbH^2$ is monotonically non-increasing. This implies that the sequence $\{{\textbf w}_n^k\}_{k=1}^K$ generated by GADMM converges to  ${\textbf w}_n^\star$ for all $n$ as $K\rightarrow\infty$ in the $\bbH$-norm.  
Finally, from the fact that $\sum_{k=1}^\infty \norm{{\textbf w}_n^{k+1} -  {\textbf w}_n^{k}}_\bbH^2 < \infty$ and $\sum_{n \in {\cal N}_t}\norm{{\textbf w}_n^{k+1} -  {\textbf w}_n^{k}}_\bbH^2$ is monotonically non-increasing, and using  the result of Lemma \ref{lemma:convRate}, we conclude that $\sum_{n \in {\cal N}_t}\norm{{\textbf w}_n^{k+1} -  {\textbf w}_n^{k}}_\bbH^2=o(1/k)$, which is the statement of the Theorem \ref{convRateProof}.

\if0
\section{Proof of Theorem~\ref{convRateProof}: Convergence Rate of GADMM}
\label{ConvRate11}

%The convergence rate of Gauss-Seidel ADMM for sum of two separable convex functions has been studied in~\citep{lions1979splitting,he20121,he2015non}. In particular, \citep{he20121} shows a convergence rate of $O(1/k)$. Moreover, \citep{deng2017parallel} improves that results and shows a convergence rate of $o(1/k)$. In this section, we leverage and extend the proof of $o(1/k)$ convergence rate in \cite[Sec. 5]{deng2017parallel} to showing that GADMM achieves the same convergence~rate.

\colr{Consider the notation in \eqref{notation} and the definition of $\bbr_{n,n+1}^{k+1}$, we can write the result  in 
\eqref{mainIneq2} as follows
\begin{align}\label{rate:first}
\|\bbw_{k+1}-\bbw^\star\|^2_\bbH\leq &\|\bbw_{k}-\bbw^\star\|^2_\bbH-
\frac{1}{\rho}\sum_{n=1}^{N-1} \norm{\lamb_{n}^{k+1} - \lamb_{n}^{k}}^2\nonumber 
\\
&-\sum_{n\in {\cal N}_h\setminus\{1\}} \rho\norm{ \boldsymbol{\theta}_{n-1}^{k+1} -  \boldsymbol{\theta}_{n-1}^k}^2-\sum_{n\in {\cal N}_h}\rho\norm{ \boldsymbol{\theta}_{n+1}^{k+1} -  \boldsymbol{\theta}_{n+1}^k}^2.
\end{align}
Further, from the definition of $\bbw_k$ and the notation in \eqref{notation}, we can write
\begin{align}\label{rate:2}
\|\bbw_{k+1}-\bbw^\star\|^2_\bbH\leq &\|\bbw_{k}-\bbw^\star\|^2_\bbH-\|\bbw_{k+1}-\bbw_{k}\|^2_\bbH.
\end{align}
The result in \eqref{rate:2} shows that the iterate sequence $\bbw_k$ obtained by the GADMM algorithm is strictly contractive. This implies that the sequence $\|\bbw_{k}-\bbw^\star\|^2_\bbH$ is monotonically decreasing as $k\rightarrow\infty$. This result implies the convergence of the iterates $\bbw_k$ from the contraction methods \citep{He1997}. 
To prove the convergence rate using the Lemma \ref{lemma:convRate}, we define the sequence $a_k:=\|\bbw_{k+1}-\bbw^\star\|^2_\bbH$. In order to apply the results of Lemma \ref{lemma:convRate}, we need to prove that 
i) $a_k$ sequence is positive which is trivial from the definition,
ii) $a_k$ is monotonically non-increasing,
iii) and $a_k$ is summable.}
For the sequence ${\textbf w}_n$, I think its difficult to prove the third point, hence we cannot use Lemma 3. We can prove these three properties for ${\textbf w}_n^k$
Let us define ${\textbf w}_n$ for all $n \in {\cal N}_t$ and $\bbH$ as follows:
\begin{align}\label{definitions}
{\textbf w}_n:=\begin{bmatrix} 
\boldsymbol{\theta}_n\\
-\lamb_{n-1}\\
\lamb_{n}\\
\end{bmatrix}
,\bbH:=\begin{bmatrix} 
\rho \bbA_n^T\bbA_n& \\
& \frac{1}{\rho}\bbI\\
&& \frac{1}{\rho}\bbI\\
\end{bmatrix},
\end{align}
where, $\bbA_{n \in  {\cal N}_t} \in \mathbb{R}^{(N-1)\times d}$ is the sub-matrix of the $n$-th element when the constraints in \eqref{com_admm_c1} are written in the matrix form, and $\bbI \in \mathbb{R}^{(N-1)\times(N-1)}$ is the identity matrix.
From the definitions in \eqref{definitions}, it holds that
\begin{align}
\!\!\!\!\!\!\!\!\sum_{n \in {\cal N}_t}\Big[\!\norm{{\textbf w}_n^{k} \!-\!  {\textbf w}_n^\star}_\bbH^2\!-\norm{ {\textbf w}_n^{k+1} \!\!-\!  {\textbf w}_n^\star}_\bbH^2\Big]&\!\!=\!\!\sum_{n} 1/\rho\left(\norm{ \lamb_n^{k}-\lamb_n^\star}^2-\norm{\lamb_n^{k+1}-\lamb_n^\star}^2\right)\nonumber
\\
&\quad+\!\!\sum_{n\in {\cal N}_t}\rho\left(\norm{\boldsymbol{\theta}_{n}^{k} -  \boldsymbol{\theta}^\star}^2- \norm{\boldsymbol{\theta}_{n}^{k+1} -  \boldsymbol{\theta}^\star}^2\right)
\label{convRateEq1}
\end{align}
where $\norm{\bbx}_{\bbH}^2=\ip{\bbx,\bbH\bbx}$. However, the following holds true for the second term on the right hand side of \eqref{convRateEq1}
\begin{align}\label{convRateEq2}
\sum_{n\in {\cal N}_t}\rho\left(\norm{\boldsymbol{\theta}_{n}^{k} -  \boldsymbol{\theta}^\star}^2- \norm{\boldsymbol{\theta}_{n}^{k+1} -  \boldsymbol{\theta}^\star}^2\right)
\!\!=\!\!\!&\!\!\!\!\sum_{n\in {\cal N}_h\setminus\{1\}}\rho\left( \norm{\boldsymbol{\theta}_{n-1}^{k} -  \boldsymbol{\theta}^\star}^2- \norm{\boldsymbol{\theta}_{n-1}^{k+1} -  \boldsymbol{\theta}^\star}^2\right)\nonumber
\\
&\quad\quad+\sum_{n\in {\cal N}_h}\rho\left(\norm{\boldsymbol{\theta}_{n+1}^{k} -  \boldsymbol{\theta}^\star}^2-\norm{ \boldsymbol{\theta}_{n+1}^{k+1} -  \boldsymbol{\theta}^\star}^2\right).
\end{align}
Therefore, the right hand side of \eqref{convRateEq1} reduces to 
\begin{align}\label{convRateEq3}
\!\!\!\!\!\!\!\!\sum_{n \in {\cal N}_t}\Big[\!\norm{{\textbf w}_n^{k} \!-\!  {\textbf w}_n^\star}_\bbH^2\!-\norm{ {\textbf w}_n^{k+1} \!\!-\!  {\textbf w}_n^\star}_\bbH^2\Big]&\!\!=\!\!\sum_{n} 1/\rho\left(\norm{ \lamb_n^{k}-\lamb_n^\star}^2-\norm{\lamb_n^{k+1}-\lamb_n^\star}^2\right)
\\
&\quad+\sum_{n\in {\cal N}_h\setminus\{1\}}\rho\left( \norm{\boldsymbol{\theta}_{n-1}^{k} -  \boldsymbol{\theta}^\star}^2- \norm{\boldsymbol{\theta}_{n-1}^{k+1} -  \boldsymbol{\theta}^\star}^2\right)\nonumber
\\
&\quad\quad+\sum_{n\in {\cal N}_h}\rho\left(\norm{\boldsymbol{\theta}_{n+1}^{k} -  \boldsymbol{\theta}^\star}^2-\norm{ \boldsymbol{\theta}_{n+1}^{k+1} -  \boldsymbol{\theta}^\star}^2\right). \nonumber
\end{align}
However, from \eqref{mainIneq} in the proof of Theorem \ref{theorem}, it holds that all the three terms on the right hand side of equality in \eqref{convRateEq3} are monotonically non-increasing. Hence,  the term $\sum_{n \in {\cal N}_t}\norm{{\textbf w}_n^{k+1} -  {\textbf w}_n^{k}}_\bbH^2$ is monotonically non-increasing. This implies that the sequence $\{{\textbf w}_n^k\}_{k=1}^K$ generated by GADMM converges to  ${\textbf w}_n^\star$ for all $n$ as $K\rightarrow\infty$ in the $\bbH$-norm.  
Finally, from the fact that $\sum_{k=1}^\infty \norm{{\textbf w}_n^{k+1} -  {\textbf w}_n^{k}}_\bbH^2 < \infty$ (\colr{Can we prove this, if this is done, then we are good to go.}) and $\sum_{n \in {\cal N}_t}\norm{{\textbf w}_n^{k+1} -  {\textbf w}_n^{k}}_\bbH^2$ is monotonically non-increasing, and using  the result of Lemma \ref{lemma:convRate}, we conclude that $\sum_{n \in {\cal N}_t}\norm{{\textbf w}_n^{k+1} -  {\textbf w}_n^{k}}_\bbH^2=o(1/k)$, which is the statement of the Theorem \ref{convRateProof}.
\fi
